# Supplementary material for: Transparent electrodes based on mixtures of nanowires and nanorings: A mean-field approach along with computer simulation
Source: arXiv:2211.04055 ancillary file (2022-11-29)
Supplement: Supplementary file 1 [file RingsANDsticksSM.pdf]

# Supplementary Materials. Transparent electrodes based on a mixture of wanowires and nanorings

Yuri Yu. Tarasevich[a)] and Andrei V. Eserkepov[b)]
*Laboratory of Mathematical Modeling, Astrakhan State University, Astrakhan, 414056, Russia*

(Dated: 3 November 2022)

## I. INTERSECTION OF A STICK AND A RING

Consider a ring of radius $r$ and a segment (zero-width stick) of length $l$. Let the origin of coordinates is located in the center of the circle, while the abscissa goes from the center of the circle through the center of the segment. Then the coordinates of the center of the segment are $(x_\mathrm{s}, 0)$. We denote the angle between the direction of the segment and the direction of the abscissa axis as $\alpha/2$ ($k = \tan\frac{\alpha}{2}$). Let there be a line and the segment lies on this line (Fig. 1).

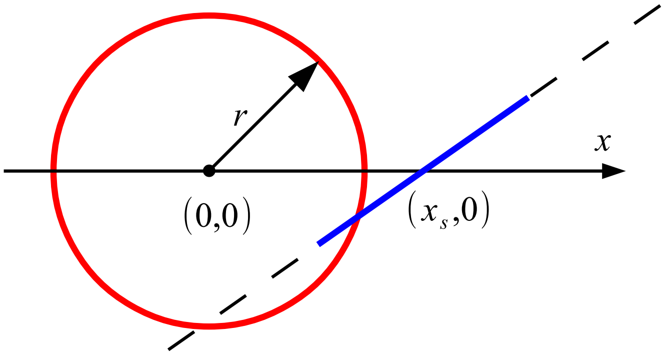


FIG. 1. Ring and segment.

With this choice of coordinate system, the circle equation is

$$x^2 + y^2 = r^2, \tag{1}$$

while line equation is

$$y = k(x - x_\mathrm{s}). \tag{2}$$

The coordinates of the intersection points of the circle and the line can be found from the equation

$$x^2 + \left[k(x - x_\mathrm{s})\right]^2 = r^2.$$

$$x_{1,2} = \frac{k^2 x_\mathrm{s} \pm \sqrt{D}}{1 + k^2}, \quad D = \left(1 + k^2\right) r^2 - k^2 x_\mathrm{s}^2.$$

The line intersect the circle when

$$\left(1 + k^2\right) r^2 - k^2 x_\mathrm{s}^2 \geqslant 0.$$

For a segment to intersect a circle, the following conditions must be met

$$|x_\mathrm{s} - x_i| \leqslant \frac{l}{2} \cos\frac{\alpha}{2}, \quad i = 1, 2.$$

---

a) Corresponding author: tarasevich@asu.edu.ru
b) Electronic mail: dantealigjery49@gmail.com

An analysis of all possible situations lead to the following results.

The case when $l > 2r$.

If

$$x > r + \frac{l}{2},$$

the segment cannot intersect the circle.

If

$$\sqrt{r^2 + \left(\frac{l}{2}\right)^2} \leqslant x \leqslant r + \frac{l}{2},$$

the segment intersects the circle only once when

$$\alpha \leqslant 2 \arccos \frac{l^2 - 4r^2 + 4x^2}{4lx}.$$

if

$$r \leqslant x < \sqrt{r^2 + \left(\frac{l}{2}\right)^2},$$

the segment intersects the circle only once when

$$\alpha < 2 \arccos \frac{l^2 - 4r^2 + 4x^2}{4lx}$$

or twice when

$$2 \arccos \frac{l^2 - 4r^2 + 4x^2}{4lx} \leqslant \alpha < 2 \arcsin \frac{r}{x}.$$

If

$$\frac{l}{2} - r < x < r,$$

the segment intersects the circle only once when

$$\alpha < 2 \arccos \frac{l^2 - 4r^2 + 4x^2}{4lx},$$

or twice when

$$\alpha \geqslant 2 \arccos \frac{l^2 - 4r^2 + 4x^2}{4lx}.$$

if

$$x \leqslant \frac{l}{2} - r,$$

the segment intersects the circle twice for any value of $\alpha$.

The probability that a line segment and a circle have one intersection point is

$$P_1 = \frac{1}{\pi L^2} \int_{\frac{l}{2}-r}^{\frac{l}{2}+r} 2 \arccos \frac{l^2 - 4r^2 + 4x^2}{4lx} (2\pi x) \, \mathrm{d}x = 2\pi \left(\frac{r}{L}\right)^2.$$

The probability that a line segment and a circle have two intersection points is

$$P_2 = \frac{1}{\pi L^2} \int_0^{\frac{l}{2}-r} (2\pi x)\pi \, \mathrm{d}x + \frac{1}{\pi L^2} \int_{\frac{l}{2}-r}^{r} \left(\pi - 2 \arccos \frac{l^2 - 4r^2 + 4x^2}{4lx}\right) 2\pi x \, \mathrm{d}x +$$
$$\frac{1}{\pi L^2} \int_r^{\sqrt{r^2+\left(\frac{l}{2}\right)^2}} \left(2 \arcsin \frac{r}{x} - 2 \arccos \frac{l^2 - 4r^2 + 4x^2}{4lx}\right) 2\pi x \, \mathrm{d}x,$$

$$P_2 = \frac{2lr - \pi r^2}{L^2}.$$

The case when $l \leqslant 2r$. If

$$x < r - \frac{l}{2},$$

the segment cannot intersect the circle.

If

$$r - \frac{l}{2} \leqslant x < \sqrt{r^2 - \left(\frac{l}{2}\right)^2},$$

the segment intersects the circle only once when

$$\alpha < 2\pi - 2\arccos\frac{l^2 - 4r^2 + 4x^2}{4lx}.$$

If

$$\sqrt{r^2 - \left(\frac{l}{2}\right)^2} \leqslant x < r,$$

the segment intersects the circle only once when

$$\alpha < 2\arccos\frac{l^2 - 4r^2 + 4x^2}{4lx},$$

or twice when

$$\alpha \geqslant 2\arccos\frac{l^2 - 4r^2 + 4x^2}{4lx}.$$

If

$$r \leqslant x < \sqrt{r^2 + \left(\frac{l}{2}\right)^2},$$

the segment intersects the circle only once when

$$\alpha < 2\arccos\frac{l^2 - 4r^2 + 4x^2}{4lx},$$

or twice when

$$2\arccos\frac{l^2 - 4r^2 + 4x^2}{4lx} \leqslant \alpha < 2\arcsin\frac{r}{x}.$$

If

$$\sqrt{r^2 + \left(\frac{l}{2}\right)^2} \leqslant x \leqslant r + \frac{l}{2},$$

the segment intersects the circle only once when

$$\alpha \leqslant 2\arccos\frac{l^2 - 4r^2 + 4x^2}{4lx}.$$

If

$$x > r + \frac{l}{2},$$

the segment cannot intersect the circle.

The probability that a line segment and a circle have one intersection point is

$$P_1 = \frac{1}{\pi L^2} \int_{r-\frac{l}{2}}^{\sqrt{r^2-\left(\frac{l}{2}\right)^2}} \left(2\pi - 2\arccos\frac{l^2-4r^2+4x^2}{4lx}\right)(2\pi x)\,\mathrm{d}x + \frac{1}{\pi L^2}\int_{\sqrt{r^2-\left(\frac{l}{2}\right)^2}}^{r+\frac{l}{2}} 2\arccos\frac{l^2-4r^2+4x^2}{4lx}(2\pi x)\,\mathrm{d}x,$$

$$P_1 = \frac{4r^2}{L^2}\left(\arcsin z + z\sqrt{1-z^2}\right), \quad z = \frac{l}{2r},$$

The probability that a line segment and a circle have two intersection points is

$$P_2 = \frac{1}{\pi L^2}\int_{\sqrt{r^2-\left(\frac{l}{2}\right)^2}}^{r}\left(\pi - 2\arccos\frac{l^2-4r^2+4x^2}{4lx}\right)2\pi x\,\mathrm{d}x + $$

$$+\frac{1}{\pi L^2}\int_{r}^{\sqrt{r^2+\left(\frac{l}{2}\right)^2}}\left(2\arcsin\frac{r}{x} - 2\arccos\frac{l^2-4r^2+4x^2}{4lx}\right)2\pi x\,\mathrm{d}x,$$

$$P_2 = \frac{r^2}{L^2}\left(4z - 2\arcsin z - 2z\sqrt{1-z^2}\right), \quad z = \frac{l}{2r}.$$
